# Supplementary material for: Megahertz-rate Ultrafast X-ray Scattering and Holographic Imaging at the European XFEL
Source: arXiv:2201.06350 ancillary file (2022-01-20)
Supplement: Supplementary file 1 [file EuXFEL_SCS_SI.pdf]

# MHz-rate Ultrafast X-ray Scattering and Holographic Imaging at the European XFEL

## Supplementary Information

### I. SCS INSTRUMENT FEATURES

|                               |                                                                                      |
|-------------------------------|--------------------------------------------------------------------------------------|
| Photon energy                 | 0.25 keV to 3 keV                                                                    |
| Relative photon bandwidth     | 0.5%                                                                                 |
| X-ray pulse energy            | $\leq 10$ mJ                                                                         |
| X-ray pulse duration          | 1 fs to 100 fs (FWHM)                                                                |
| Polarization                  | Linear. Elliptical with thin film polarizers.                                        |
| Focal spot size on the sample | From 1 $\mu\text{m}$ (horizontal) or 2 $\mu\text{m}$ (vertical) to 500 $\mu\text{m}$ |
| Magnetic field                | DC electromagnet $\leq 0.5$ T                                                        |
| Optical laser systems         | 800 nm: $\leq 1$ mJ, 15 fs to 100 fs<br>1030 nm: $\leq 20$ mJ, 850 fs                |

TABLE I. Key features of the SCS instrument available for the experiments described in the main text. Future developments are not discussed in the current manuscript.

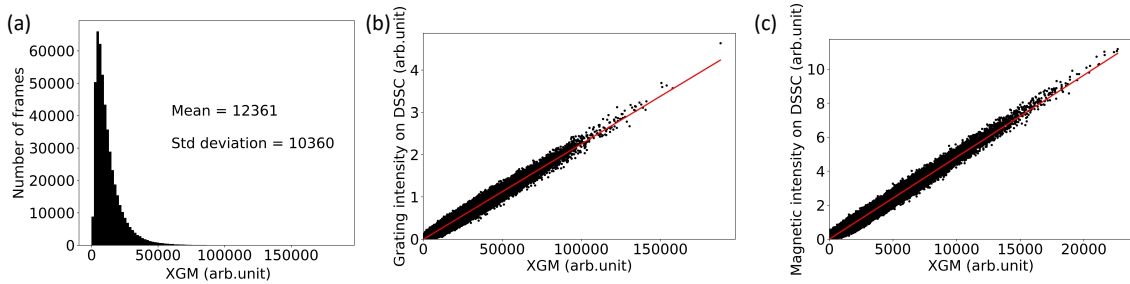

FIG. 1. X-ray pulse intensity fluctuation and correlation with the DSSC detector data.

(a) Histogram of the single-shot X-ray intensities within one typical acquisition run containing  $5 \cdot 10^5$  pulses measured with the XGM  $I_0$  detector. (b) Symbols: charge scattering amplitude from a curved grating measured on the DSSC detector as a function of  $I_0$ . Solid line: linear regression on the data. (c) Symbols: magnetic scattering amplitude from magnetic domains measured on the DSSC detector as a function of  $I_0$ . Solid line: linear regression on the data.

## II. DSSC–XGM INTENSITY CORRELATION

The X-ray pulses produced at XFELs based on the SASE mechanism have intrinsic intensity fluctuations due to the stochastic nature of the SASE process [1]. For this reason, it is important to monitor the incoming pulse intensity  $I_0$  on a shot-to-shot basis using an XGM, and properly normalize the 2D detector signal. A histogram of  $I_0$  measured by the XGM for a typical XFEL run is shown in Fig. 1(a). One can clearly see that the standard deviation of the curve is comparable to its mean, which justifies the need for a shot-to-shot normalization. In addition, since two different detectors are used to measure the incoming and the scattered X-ray intensity, it must be ensured that both operate in a regime away from intrinsic nonlinearities, which are typically different for different detectors. In Fig. 1(b)-(c) we show the intensity correlation between the DSSC detector and the  $I_0$  monitor for two types of samples. In Fig. 1(b), we used custom-built curved gratings [2], which created a pair of isolated scattering features on the DSSC. The y-axis is the integrated intensity over a suitable region of the detector which contains those isolated features. In Fig. 1(c) instead, we used a sample comprising labyrinth magnetic domains producing a ring-like scattering pattern on the DSSC detector. The y-axis in this case is the azimuthally integrated intensity over the entire ring. For both the curved grating and the magnetic domain sample, with one order of magnitude different  $I_0$  values, the XGM and DSSC detectors show a clear linear correlation. This indicates that normalization of the DSSC data with the XGM signal is reliable, opening the way to high quality spectroscopy experiments not achievable at earlier XFELs.

### III. TIME-RESOLVED SAXS SAMPLE DETAILS

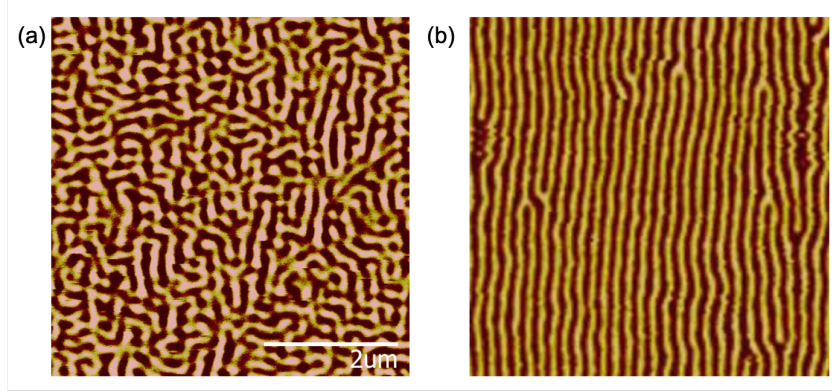

FIG. 2. (a) 5  $\mu\text{m}$  x 5  $\mu\text{m}$  MFM images of the CoFe/Ni multilayer. (b) Example of a MFM image of stripe domains aligned with an external in-plane magnetic field.

Figure 2(a) shows the MFM of the Ta(3 nm) / Cu(5 nm) / [CoFe(0.25 nm)-Ni(0.75 nm)]<sub>20</sub> / CoFe(0.25 nm) / Cu(3 nm) / Ta(3 nm) multilayer sample. This image shows randomly oriented labyrinth domains. Those were aligned into stripes with an in-plane magnetic field. A typical MFM image of the stripe domains obtained in this way is shown in Fig. 2(b).

### IV. X-RAY HOLOGRAPHY SAMPLE DETAILS

Figure 3(a) illustrates a MFM image of the [Ta(5 nm)/Co<sub>20</sub>Fe<sub>60</sub>B<sub>20</sub>(0.9 nm)/MgO(2 nm)]<sub>15</sub> multilayer sample. Figure 3(b) shows a SEM image of the holography mask. The mask is a square with a 2.5  $\mu\text{m}$  side, rotated by 45° with respect to membrane's side. The holography mask has also two orthogonal slits for encoding the reference beam, according to the HERALDO technique [3].

### V. RECONSTRUCTION USING THE HERALDO TECHNIQUE

In this section we show the impact of the inactive areas of the DSSC on the holographic image reconstruction. Fig 4(a) shows the hologram recorded at the SOLEIL synchrotron mapped with the gaps of the DSSC and the corresponding reconstructed image is shown in Fig 4(b). While the gaps generally affect the reconstruction, this holography mask was specifically designed to minimize their impact, as clearly shown in the figure. A more crucial aspect for the reconstruction is the correct placement of the 16 independent ladders of the detector, since a small displacement of one single ladders can severely distort the reconstruction from Fourier

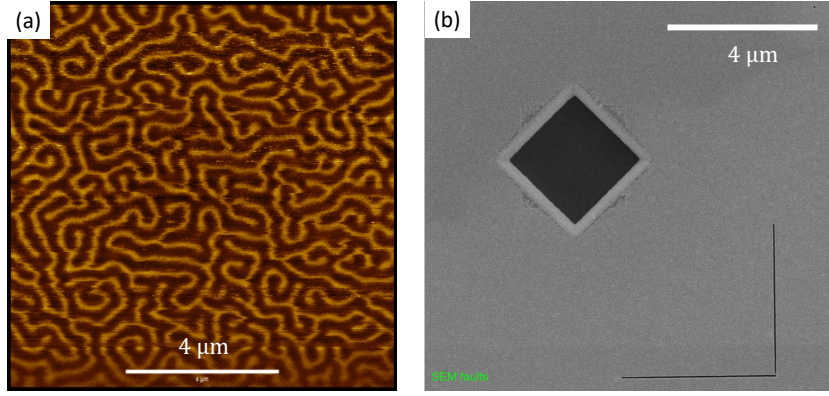

FIG. 3. (a)  $10\ \mu\text{m} \times 10\ \mu\text{m}$  MFM image of the CoFeB multilayer sample discussed in the main text. (b) Scanning Electron Microscope (SEM) image of the holography mask.

transform. A on-time systematic and careful procedure to manually align the quadrants using the characteristic features of the scattering was required ahead of the first reconstruction, but once the detector is aligned, it is ready for all subsequent data and experiments.

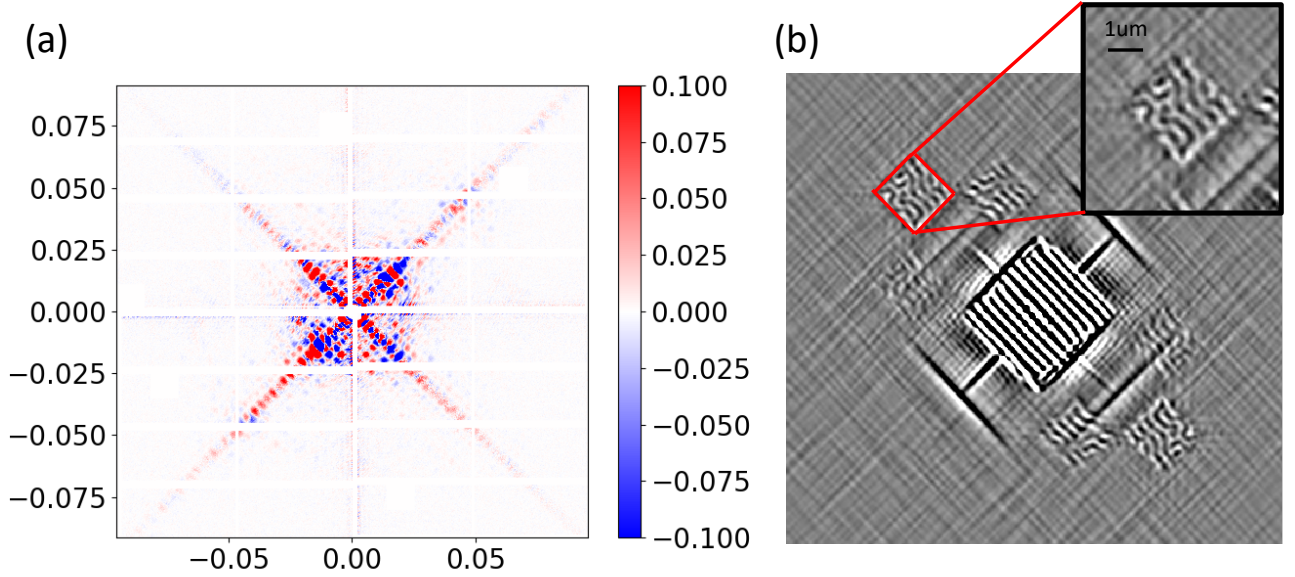

FIG. 4. (a) Hologram recorded at the COMET-end station at the SOLEIL synchrotron masked with the gaps of the DSSC detector. (b) Reconstructions of the magnetic domains using the HERALDO technique.

## VI. HEAT DIFFUSION SIMULATION DETAILS

The parameters used for the heat diffusion simulation are summarized in Table II. In addition to those, the thermal conductance of the layer-to-layer interfaces are assumed to be  $2 \times 10^9 \text{ W m}^{-2} \text{ K}^{-1}$  for the metal-metal and  $0.3 \times 10^9 \text{ W m}^{-2} \text{ K}^{-1}$  for the metal-insulator cases [4–6].

|                         | $n$          | $k$          | $\beta$ [7]           | Thermal<br>conductivity<br>$\text{W m}^{-1} \text{ K}^{-1}$ | Heat<br>capacity<br>$\text{J kg}^{-1} \text{ K}^{-1}$ | Density<br>$\text{kg m}^{-3}$ |
|-------------------------|--------------|--------------|-----------------------|-------------------------------------------------------------|-------------------------------------------------------|-------------------------------|
| Ta                      | 1.11 [8]     | 3.48 [8]     | $1.26 \times 10^{-3}$ | 57.5                                                        | 140                                                   | 16690                         |
| Cu                      | 0.105 [9]    | 5.14 [9]     | $2.97 \times 10^{-3}$ | 41 [10]                                                     | 385                                                   | 8960                          |
| [CoFe/Ni] <sub>20</sub> | 2.49 [11–13] | 4.51 [11–13] | $1.96 \times 10^{-3}$ | 42.8 [14, 15]                                               | 435                                                   | 8877                          |
| Si                      | 3.67 [16]    | 0.005 [16]   | $9.46 \times 10^{-5}$ | 10 [17]                                                     | 691 [18]                                              | 2329                          |
| Au                      | 0.18 [12]    | 5.15 [12]    | $1.95 \times 10^{-3}$ | 244.3 [19]                                                  | 129                                                   | 19300                         |

TABLE II. Parameters used for the heat diffusion simulation. The refractive index  $n$  and extinction coefficient  $k$  is for 800 nm wavelength, while the X-ray extinction coefficient  $\beta$  is taken for the photon energy of the cobalt  $L_3$  edge 778.8 eV. The parameters of the [CoFe(0.25 nm) / Ni(0.75 nm)]<sub>20</sub> multilayer sample have been extrapolated using the parameters of the single constituting elements.

- 
- [1] E. L. Saldin, E. A. Schneidmiller, and M. V. Yurkov, New Journal of Physics **12**, 035010 (2010), ISSN 1367-2630, URL <https://doi.org/10.1088/1367-2630/12/3/035010>.
  - [2] M. Schneider, C. M. Günther, C. v. K. Schmising, B. Pfau, and S. Eisebitt, Optics Express **24**, 13091 (2016), ISSN 1094-4087, URL <https://www.osapublishing.org/oe/abstract.cfm?uri=oe-24-12-13091>.
  - [3] D. Zhu, M. Guizar-Sicairos, B. Wu, A. Scherz, Y. Acremann, T. Tyliczszak, P. Fischer, N. Friedberger, K. Ollefs, M. Farle, et al., Physical Review Letters (2010), ISSN 00319007.
  - [4] H.-K. Lyo and D. G. Cahill, Phys. Rev. B **73**, 144301 (2006), URL <https://link.aps.org/doi/10.1103/PhysRevB.73.144301>.
  - [5] R. M. Costescu, M. A. Wall, and D. G. Cahill, Phys. Rev. B **67**, 054302 (2003), URL <https://link.aps.org/doi/10.1103/PhysRevB.67.054302>.

- [6] B. C. Gundrum, D. G. Cahill, and R. S. Averback, Phys. Rev. B **72**, 245426 (2005), URL <https://link.aps.org/doi/10.1103/PhysRevB.72.245426>.
- [7] B. L. Henke, E. M. Gullikson, and J. C. Davis, Atomic Data and Nuclear Data Tables **54**, 181 (1993), ISSN 0092-640X, URL <https://www.sciencedirect.com/science/article/pii/S0092640X83710132>.
- [8] M. A. Ordal, R. J. Bell, R. W. Alexander, L. A. Newquist, and M. R. Query, Appl. Opt. **27**, 1203 (1988), URL <http://www.osapublishing.org/ao/abstract.cfm?URI=ao-27-6-1203>.
- [9] K. M. McPeak, S. V. Jayanti, S. J. P. Kress, S. Meyer, S. Iotti, A. Rossinelli, and D. J. Norris, ACS Photonics **2**, 326 (2015), URL <https://doi.org/10.1021/ph5004237>.
- [10] A. D. Avery, S. J. Mason, D. Bassett, D. Wesenberg, and B. L. Zink, Phys. Rev. B **92**, 214410 (2015), URL <https://link.aps.org/doi/10.1103/PhysRevB.92.214410>.
- [11] M. A. Ordal, R. J. Bell, R. W. Alexander, L. L. Long, and M. R. Query, Appl. Opt. **24**, 4493 (1985), URL <http://www.osapublishing.org/ao/abstract.cfm?URI=ao-24-24-4493>.
- [12] M. A. Ordal, R. J. Bell, R. W. Alexander, L. L. Long, and M. R. Query, Appl. Opt. **26**, 744 (1987), URL <http://www.osapublishing.org/ao/abstract.cfm?URI=ao-26-4-744>.
- [13] P. B. Johnson and R. W. Christy, Phys. Rev. B **9**, 5056 (1974), URL <https://link.aps.org/doi/10.1103/PhysRevB.9.5056>.
- [14] S. Srichandan, phd (2018).
- [15] S. F.-Y. ZHU Li-Dan and S. F.-Y. ZHU Li-Dan, Chinese Physics Letters **29**, 66301 (2012), ISSN 0256-307X, URL <http://cpl.iphy.ac.cn/EN/10.1088/0256-307X/29/6/066301>.
- [16] C. Schinke, P. Christian Peest, J. Schmidt, R. Brendel, K. Bothe, M. R. Vogt, I. Kröger, S. Winter, A. Schirmacher, S. Lim, et al., AIP Advances **5**, 067168 (2015), <https://doi.org/10.1063/1.4923379>, URL <https://doi.org/10.1063/1.4923379>.
- [17] A. McConnell, S. Uma, and K. Goodson, Journal of Microelectromechanical Systems **10**, 360 (2001).
- [18] J. Kimling, A. Philippi-Kobs, J. Jacobsohn, H. P. Oepen, and D. G. Cahill, Phys. Rev. B **95**, 184305 (2017), URL <https://link.aps.org/doi/10.1103/PhysRevB.95.184305>.
- [19] G. Chen and P. Hui, Applied Physics Letters **74**, 2942 (1999), <https://doi.org/10.1063/1.123973>, URL <https://doi.org/10.1063/1.123973>.
